# Supplementary material for: Automated adaptive inference of coarse-grained dynamical models in systems biology
Source: arXiv:1404.6283 source file (2014-04-24)

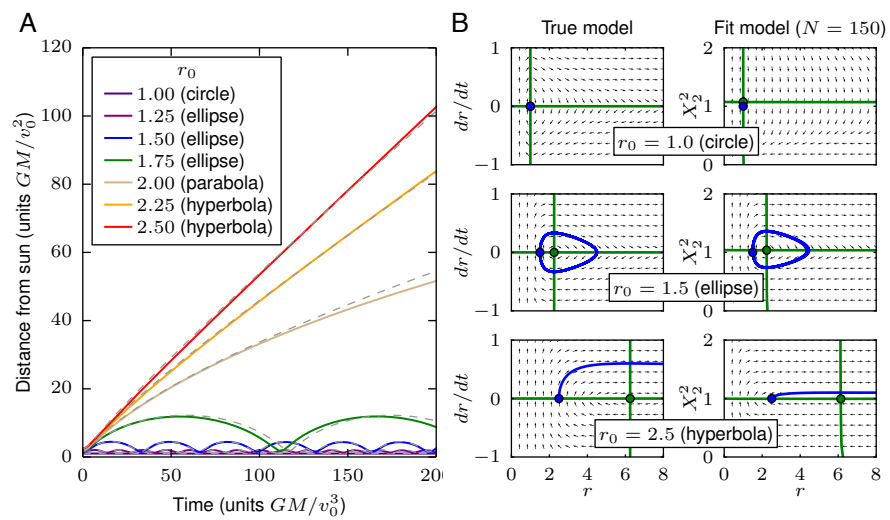

More nonlinearities

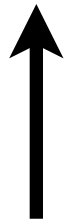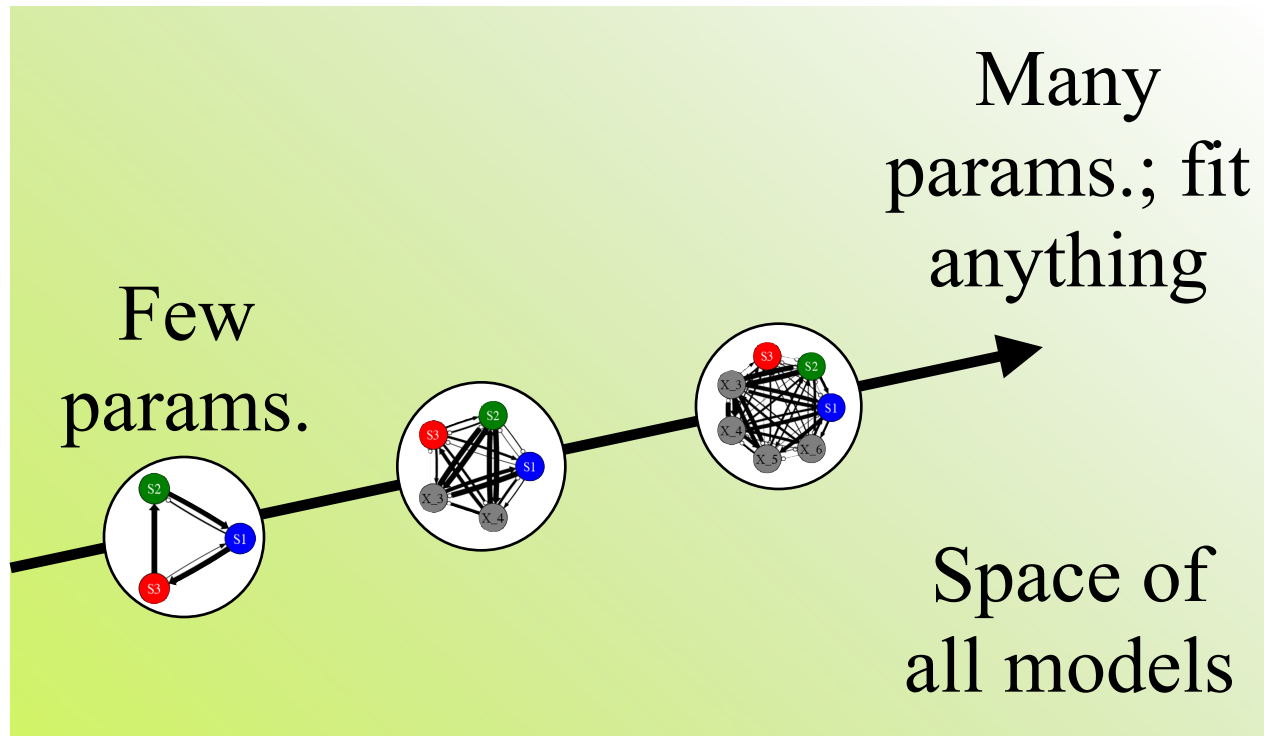

Few  
params.

Many  
params.; fit  
anything

Space of  
all models

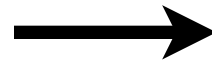

More hidden variables

## In-sample data

### Planetary motion

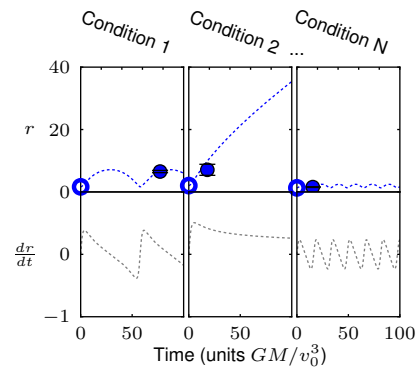

### Multi-site phosphorylation

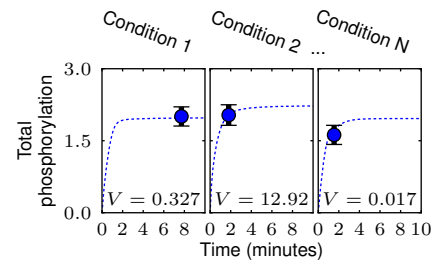

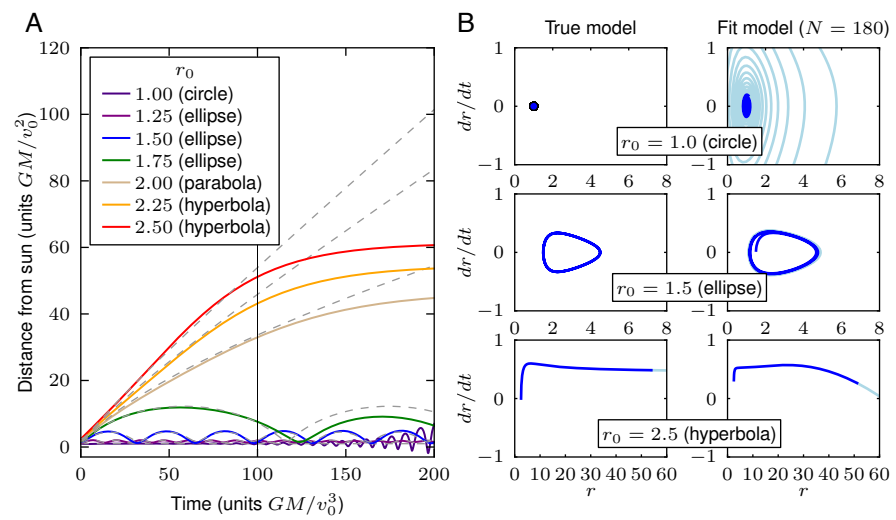

## chi^2 vs. N

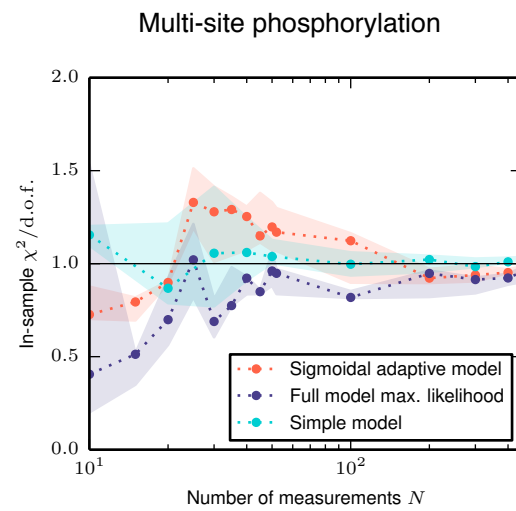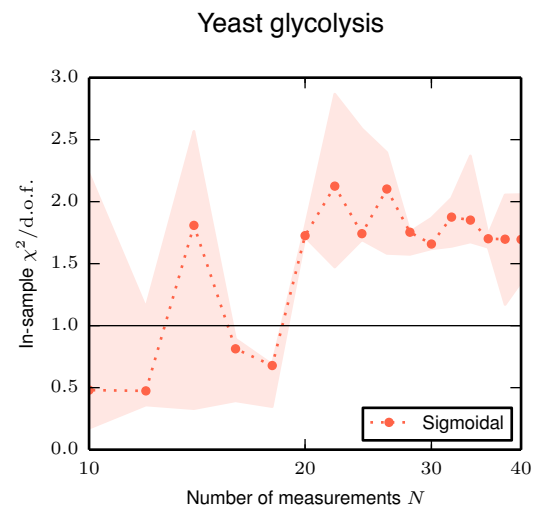

yeast\_networkFigure\_original.pdf

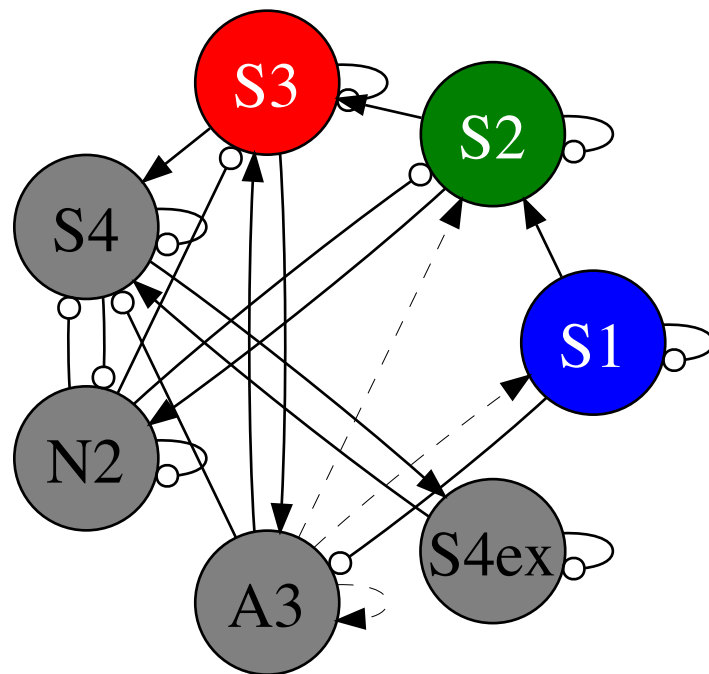

131111\_complexExample\_network\_smallFont\_Model 9.pdf

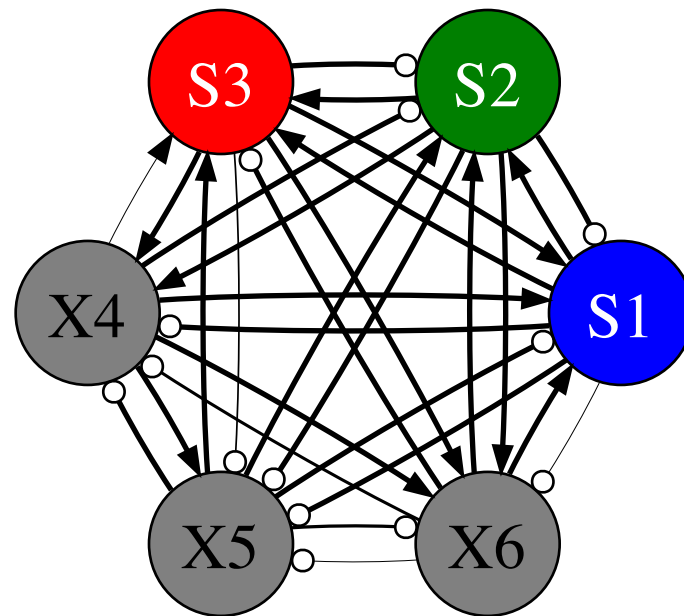

For planetary motion:  
fit model has lower  $\chi^2$   
(means fitting algorithm is  
working)

# Yeast glycolysis model selection as function of $N$

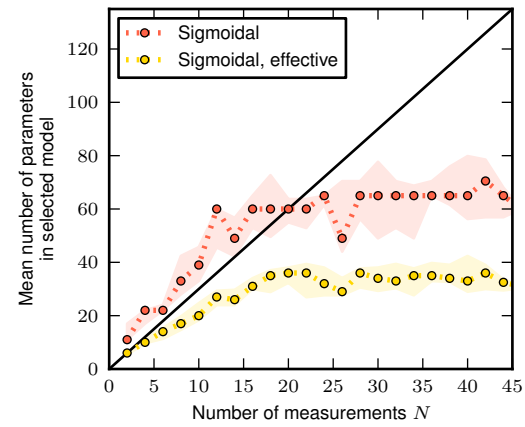



## Scaling of computational effort

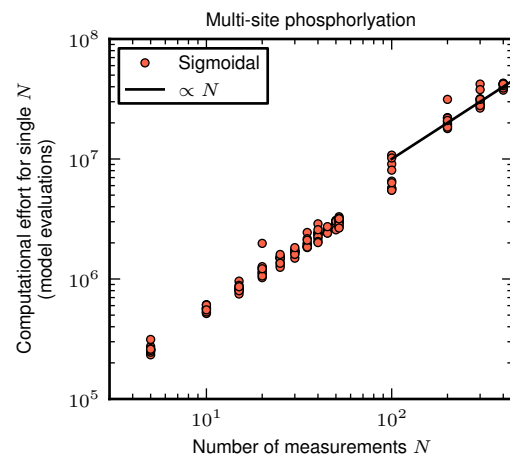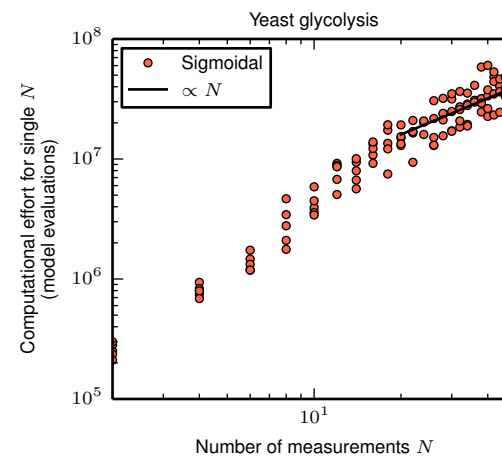

Supplement: Supplementary file 1 [file appendix_paperFigures.pdf]
